# Supplementary material for: FIGARO: Improving System Performance via Fine-Grained In-DRAM Data Relocation and Caching
Source: arXiv:2009.08437 source file (2020-09-17)
Supplement: Supplementary file 1 [file appendix.tex]

\appendix

\section{Tables}

\begin{table}[htbp]
  \centering
  \caption{Add caption}
  \resizebox{\linewidth}{!}{
    \begin{tabular}{lccccccc}
        \toprule
        \mr{3.5}{\emph{Module}} & \mr{3.5}{\emph{\makecell{Date\\(yy-ww)}}} &
        \multicolumn{2}{c}{\emph{Timing}} & \multicolumn{3}{c}{\emph{Organization}} & \mr{3.5}{\emph{minACT}}  \\
        \cmidrule(lr){3-4}\cmidrule(lr){5-7}
        \multicolumn{2}{c}{} & \emph{\makecell{Freq.\\(MT/s)}} & \emph{\makecell{tRC\\(ns)}} &
        \emph{\makecell{Size\\(GB)}} & \emph{Chips} & \emph{Pins} & \\
        \midrule

        \stripe
        $A_{0-2}$     & 19-19 & 2400  & 46.16 & 4     & 4     & x16   & 0 \\
        $A_{3-9}$     & 17-08 & 2133  & 47.06 & 4     & 8     & x8    & 0 \\ 
        \stripe
        $A_{10-15}$   & 19-36 & 2666  & 46.25 & 4     & 4     & x16   & 0 \\
        $A_{16-25}$   & 20-07 & 2400  & 46.16 & 8     & 8     & x8    & 0 \\
        \stripe
        $A_{26-34}$   & 19-45 & 2666  & 46.25 & 4     & 4     & x16   & 0 \\

        $B_{0-4}$     & 18-22 & 2133  & 46.5  & 4     & 8     & x8    & 0 \\
        \stripe
        $B_{5-14}$    & 43922 \todo{fix} & 2666  & 46.5  & 4     & 8     & x8    & 0 \\
        $B_{15-19}$   & 20-08 & 2133  & 46.5  & 4     & 8     & x8    & 0 \\
        \stripe
        $B_{20-24}$   & 20-08 & 2133  & 46.5  & 4     & 8     & x8    & 0 \\

        $C_{0-7}$     & 16-48 & 2133  & 46.5  & 4     & 8     & x8    & 0 \\
        \stripe
        $C_{8-15}$    & 17-12 & 2133  & 46.5  & 4     & 8     & x8    & 0 \\
        $C_{16}$      & 19-11 & 2400  & 45.75 & 4     & 4     & x16   & 0 \\
        \stripe
        $C_{17-18}$   & 19-23 & 2400  & 45.75 & 4     & 4     & x16   & 0 \\
        $C_{19-25}$   & 19-44 & 2133  & 46.5  & 8     & 8     & x8    & 0 \\
        \stripe
        $C_{26}$      & 19-06 & 2400  & 45.75 & 8     & 8     & x8    & 0 \\
        $C_{27}$      & 19-01 & 2400  & 45.75 & 8     & 8     & x8    & 0 \\
        \stripe
        $C_{28-30}$   & 19-51 & 2133  & 46.5  & 8     & 8     & x8    & 0 \\
        $X_{0-9}$ \todo{fix}     & 19-48 & 2400  & 45.75 & 8     & 8     & x8    & 0 \\
        \stripe
        $Y_{0}$ \todo{fix}       & 19-50 & 2400  & 45.75 & 8     & 8     & x8    & 0 \\
    \end{tabular}%
    } % resizebox
    \label{table:ddr4_table}%
\end{table}%

\begin{table}[htbp]
  \centering
  \caption{Add caption DDR3}
  \resizebox{\linewidth}{!}{
    \begin{tabular}{lccccccc}
        \toprule
        \mr{3.5}{\emph{Module}} & \mr{3.5}{\emph{\makecell{Date\\(yy-ww)}}} &
        \multicolumn{2}{c}{\emph{Timing}} & \multicolumn{3}{c}{\emph{Organization}} & \mr{3.5}{\emph{minACT}}  \\
        \cmidrule(lr){3-4}\cmidrule(lr){5-7}
        \multicolumn{2}{c}{} & \emph{\makecell{Freq.\\(MT/s)}} & \emph{\makecell{tRC\\(ns)}} &
        \emph{\makecell{Size\\(GB)}} & \emph{Chips} & \emph{Pins} & \\
        \midrule

        \stripe
	$A_1$ & 10-40 & 1333 & 49.5 & 2 & 8 & x8 & 0 \\ 
	$A_{2-8}$ & 14-16 & 1600 & 48.75 & 4 & 8 & x8 & 0 \\ 
        \stripe
	$A_{9-13}$ & 12-11 & 1866 & 47.91 & 2 & 8 & x8 & 0 \\ 
	$A_{14}$ & 10-19 & 1066 & 50.625 & 1 & 8 & x8 & 0 \\ 
        \stripe
	$A_{15-16}$ & 14-26/14-09 & 1600 & 48.75 & 2 & 4 & x16 & 0 \\ 
	$A_{17}$ & 15-23 & 1600 & 48.75 & 8 & 16 & x4 & 0 \\ 
        \stripe
	$A_{18-20}$ & 12-32 & 1600 & 48.75 & 2 & 8 & x8 & 0 \\ 
	$B_{1-4}$ & 15-22 & 1600 & 50.625 & 4 & 8 & x8 & 0 \\ 
        \stripe
	$B_{5-8}$ & 13-51 & 1600 & 48.75 & 4 & 8 & x8 & 0 \\ 
	$B_{9-10}$ & 10-48 & 1333 & 49.5 & 1 & 8 & x8 & 0 \\
        \stripe
	$B_{11-15}$ & 15-25 & 1600 & 48.75 & 2 & 4 & x16 & 0 \\ 
	$B_{16-18}$ & 11-42 & 1333 & 49.5 & 2 & 8 & x8 & 0 \\ 
        \stripe
	$B_{19-20}$ & 12-24 & 1600 & 48.75 & 2 & 8 & x8 & 0 \\ 
	$C_{1-7}$ & 17-03 & 1600 & ? & 4 & 8 & x8 & 0 \\ 
        \stripe
	$C_{8-12}$ & 15-46 & 1600 & ? & 2 & 8 & x8 & 0 \\ 
	$C_{13-17}$ & 10-43 & 1333 & 49.125 & 1 & 4 & x16 & 0 \\ 
        \stripe
	$C_{18}$ & 15-04 & 1600 & ? & 4 & 8 & x8 & 0 \\ 
	$C_{19}$ &  & \  & \  & \  & \  & \  & \  \\ 
        \stripe
	$C_{20}$ &  & \  & \  & \  & \  & \  & \  \\ 
    \end{tabular}%
    } % resizebox
    \label{table:ddr3_table}%
\end{table}%
